# Supplementary material for: CORSAIR: Convolutional Object Retrieval and Symmetry-AIded Registration
Source: arXiv:2103.06911 source file (2021-09-04)
Supplement: Supplementary file 1 [file Appendix.tex]

\section{Appendix}
\label{sec:appendix}
